# Supplementary material for: Evaluating Semantic Interaction on Word Embeddings via Simulation
Source: arXiv:2007.15824 source file (2020-07-31)
Supplement: Supplementary file 1 [file SI-models.pdf]

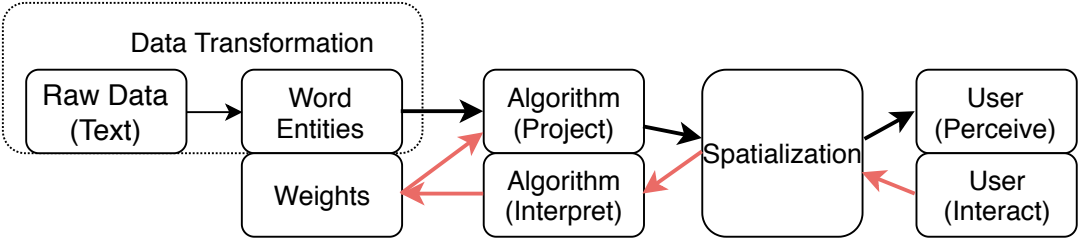

a. **Sl<sub>keyword</sub>**

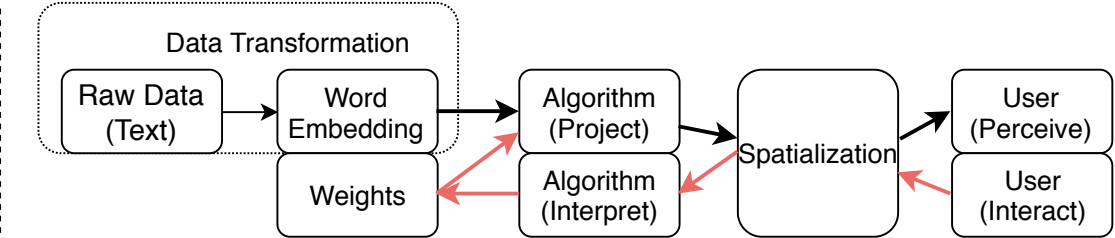

b. **Sl<sub>embedding</sub>**
